# Supplementary material for: A single-hole spin qubit
Source: arXiv:1912.10426 ancillary file (2019-12-24)
Supplement: Supplementary file 1 [file supplementary_single_hendrickx.pdf]

# Supplementary material: A single-hole spin qubit

N.W. Hendrickx,[1,*] W.I.L. Lawrie,[1] L. Petit,[1] A. Sammak,[2] G. Scappucci,[1] and M. Veldhorst[1,†]

[1]*QuTech and Kavli Institute of Nanoscience, Delft University of Technology, P.O. Box 5046, 2600 GA Delft, The Netherlands*
[2]*QuTech and Netherlands Organisation for Applied Scientific Research (TNO), Stieltjesweg 1, 2628 CK Delft, The Netherlands*

(Dated: December 20, 2019)

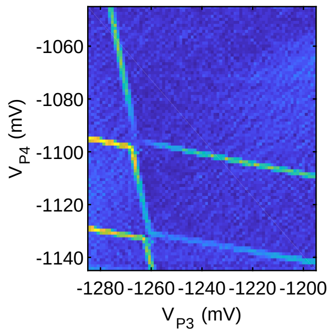


FIG. 1. **Depletion of a hole double quantum dot in germanium.** Colour map of the sensor signal as a function of the voltages on plunger gates P3 and P4. No extra addition lines can be observed beyond $V_{\mathrm{P3}} \approx -1260$ and $V_{\mathrm{P4}} \approx -1100$, indicating the double quantum dot is fully depleted. The slight decrease of voltages compared to Fig. 1 of the main text, can be attributed to a hysteretic drift as a result of extensive gate voltage sweeping.

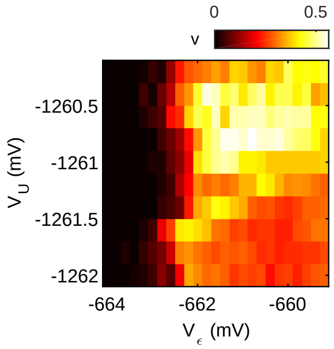


FIG. 2. **Optimisation of the readout-point.** Colour map of the visibility of the readout $v$, as defined by $v = P_{\mathrm{blocked},\pi} - P_{\mathrm{blocked},0}$, with $P_{\mathrm{blocked},\pi}$ being the probability of measuring a blocked signal after applying a resonant $\pi$-pulse to Q1 and $P_{\mathrm{blocked},0}$ the probability of measuring a blocked signal without applying any microwave pulses. A clear optimal spot for readout can be observed at $V_U = -1260.7$ mV, $V_\epsilon = -661.0$ mV.

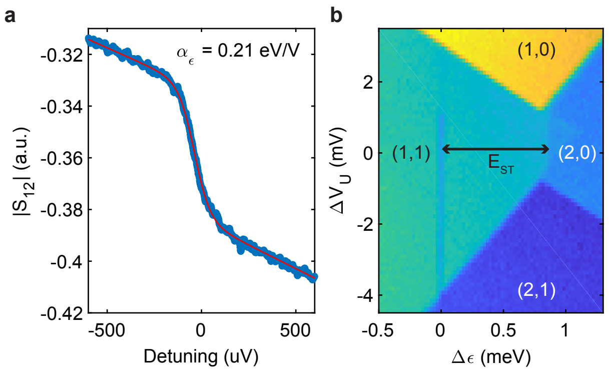


FIG. 3. **Excited state energy of the quantum dot. a** Polarisation line measurement of the (1,1)-(0,2) anticrossing. We fit the thermally limited polarisation line to a model including cross-talk to the charge sensor and the effect of the charge state on the sensor sensitivity [1]. Assuming a hole temperature of 100 mK as measured previously, we find a lever arm of $\alpha_\epsilon = 0.21$ eV/V, in good agreement with results obtained on similar devices. **b** We measure the excited state energy by applying a DC bias across the quantum dot ohmics, shifting the anti-crossing towards the negative detuning voltage. For large enough bias, the readout window is capped off, as a result of the excited state becoming available in energy. From this we deduce an excited state splitting of $E_{ST} = 0.85$ meV.

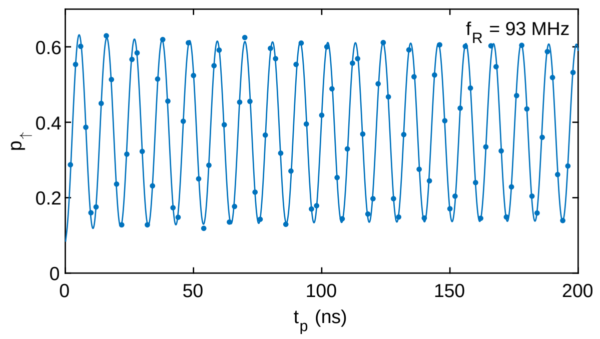


FIG. 4. **Coherent operation of Q1.** We rotate Q1 by applying a resonant microwave pulse to gate P1 and observe fast Rabi oscillations, with a frequency of $f_R = 93$ MHz.

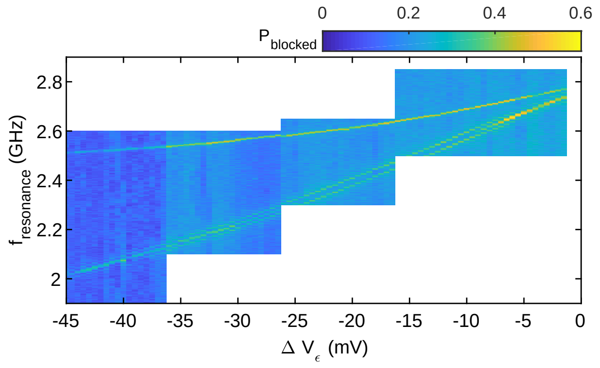


FIG. 5. **Detuning dependence of the resonance frequency of Q1 and Q2.** Colour map indicating a blocked state fraction $P_{\text{blocked}}$ as a function of the detuning voltage $\Delta V_\epsilon$ of the manipulation point. We apply a microwave pulse of $t_p = 105$ ns, corresponding to an approximate $3\pi$-pulse on Q1 and a $\pi$-pulse on Q2 at $\Delta V_\epsilon = -5$ mV. The resonance line corresponding to Q1, can be observed to split and recombine throughout the map, as a direct result of the Rabi frequency changing.

[1] L. DiCarlo, H. J. Lynch, A. C. Johnson, L. I. Childress, K. Crockett, C. M. Marcus, M. P. Hanson, and A. C. Gossard, Phys. Rev. Lett. **92**, 226801 (2004).
